# Supplementary material for: Learning to Detect Every Thing in an Open World
Source: arXiv:2112.01698 source file (2022-04-12)
Supplement: Supplementary file 2 [file tensormask_appendix.tex]

%%%%%%%%%%%%%%% Train on VOC, test on Non-VOC
\begin{table*}[t]
\centering
\resizebox{\linewidth}{!}{
\begin{tabular}{c|rrrr|rrrrrr}
\toprule
\multirow{2}{*}{Method} & \multicolumn{4}{c|}{Box}& \multicolumn{4}{c}{Mask}\\
& {\small{AP}} & \small{AR10}  & \small{AR30}  & \small{AR100}  &  {\small{AP}} & \small{AR10}  & \small{AR30}  & \small{AR100}\\
\hline 
TensorMask~\cite{chen_2019_iccv} &\textbf{9.6}&17.8&22.9&26.6&\textbf{7.4}&14.8&18.8&22.0\\
\ours &\textcolor{blue}{\small{(-0.8)}} 8.8&\textcolor{blue}{\small{(+3.0)}} \textbf{20.8}&\textcolor{blue}{\small{(+4.9)}} \textbf{27.8}&\textcolor{blue}{\small{(+7.8)}}\textbf{34.4}&\textcolor{blue}{\small{(-0.4)}} 7.0&\textcolor{blue}{\small{(+3.4)}} \textbf{18.2}&\textcolor{blue}{\small{(+5.3)}} \textbf{24.1}&\textcolor{blue}{\small{(+7.7)}} \textbf{29.7}\\ 
\bottomrule

\end{tabular}}
\vspace{-2mm}
\caption{\small{\textbf{Results of Tensormask for {VOC} $\rightarrow$ {Non-VOC} generalization in COCO}.}}
\label{tab:tensormask}
\end{table*}
